# Supplementary material for: QBitOpt: Fast and Accurate Bitwidth Reallocation during Training
Source: arXiv:2307.04535 source file (2023-07-10)
Supplement: Supplementary file 1 [file appendix_train_schedule_results.tex]

\addtolength{\tabcolsep}{-1pt}
\begin{table}[t]
\centering
\begin{tabular}{l|c|ccccc}
\toprule
Arch.  & W/A &  0\% &  25\% & 50\% & 75\% & 100\%  \\ \midrule
\multirow[c]{2}{*}{MNv2} & \mpb{4/4} & 68.63 & 69.55   &	69.71   &	 69.7	& 67.81 \\
                             & \mpb{3/3} & 62.71 & 65.83   & 65.65    &  65.56 & 62.47 \\ \midrule
\multirow[c]{2}{*}{MNv3} & \mpb{4/4} & \textcolor{magenta}{59.62} & 64.39  & 64.23     &	64.34 &62.66 \\
                                  & \mpb{3/3} & 43.70 & 57.49   & 57.14    &	56.9  & 54.94 \\ \midrule
\end{tabular}
 \caption{Comparing training \mnv{2} (MNv2) and \mnv{3}-Small (MNv3) with QBitOpt for different fractions (\%) of the total training time. This table presents the same results as Table~\ref{tbl:ablation_train_schedule_results} but includes the missing result.
 }
 \label{tbl:ablation_train_schedule_results_apendix}
\end{table}
\addtolength{\tabcolsep}{1pt}
